# Supplementary material for: Characteristic boundary conditions for Hybridizable Discontinuous Galerkin methods
Source: arXiv:2503.19684 source file (2025-03-25)
Supplement: Supplementary file 1 [file appendix.tex]

\appendix \section{Nonlinear planar acoustic pulse $\alpha = 0.5$}
\label{appendix::pulse_1d_alpha0.5}
\graphicspath{{./figures/planar_acoustic_pulse/data}}
\pgfplotsset{table/search path={./figures/planar_acoustic_pulse/data}}
\begin{figure}[htb]
    \centering
    \input{./figures/planar_acoustic_pulse/w_alpha0.5_right.tex}
    \caption[]{Incoming $\overline{w}^-$ and outgoing $\overline{w}^+$ characteristics at the boundary $\Gamma_{out}$ for a downstream propagating linear acoustic pulse with strength $\alpha = 0.5$.}
    \label{fig::w_alpha0.5_right}
\end{figure}

\begin{figure}[htb]
    \centering
    \input{./figures/planar_acoustic_pulse/w_alpha0.5_left.tex}
    \caption[]{Incoming $\overline{w}^-$ and outgoing $\overline{w}^+$ characteristics at the boundary $\Gamma_{in}$ for an upstream propagating linear acoustic pulse with strength $\alpha = 0.5$.}
    \label{fig::w_alpha0.5_left}
\end{figure}

\begin{figure}[htb]
    \centering
    \input{./figures/planar_acoustic_pulse/pulse_alpha0.5.tex}
    \caption[]{Scaled $L_2(\Omega)$-errors of the pressure $e_p$ for a linear downstream (a) and upstream (b) propagating acoustic pulse with strength $\alpha = 0.5$.}
    \label{fig::p1d_0.5}
\end{figure}
